# Supplementary material for: AExGym: Benchmarks and Environments for Adaptive Experimentation
Source: arXiv:2408.04531 source file (2024-08-08)
Supplement: Supplementary file 1 [file appendix-overview.tex]

\section*{Overview}

Code to reproduce results below is available at \href{https://github.com/namkoong-lab/AExGym.git}. {https://github.com/namkoong-lab/AExGym.git}

The appendix is organized as follows: 
\begin{itemize}
    \item Section \ref{section:dataset_details} (Dataset Details)  elaborates upon the dataset contents and setup.
    \item Section \ref{section:limitations} (Limitations) explains the existing limitations of our framework. 
    \item Section \ref{section: policies} (Policies) details the algorithms that we consider for benchmarking. 
    \item Section \ref{section: personalization} (Personalization) showcases experimental results for personalization in the Pennsylvania Reemployment Bonus Demonstration data.  
    \item Section \ref{section:site-selection} (Site Selection) continues with additional experimental results for site selection in the Meager and NHIS data. 
    \item Section \ref{section: multiple-objectives} (Multiple Objectives) details settings and results for competing objectives such as trading off between simple and cumulative regret. 
    \item Section \ref{section:constraints} (Constraints) shows experimental results for various practical constraints including budget and geographical constraints. 
    \item Section \ref{section: external-validity} (External Validity) introduces and elaborates on experiments regarding external validity methods including Optimal Experimental Design. 
    \item Section \ref{section: nonstationarity} (Non-Stationarity) shows how existing adaptive methods may fail in non-stationary environments including the ASOS and field experimental data. 
\end{itemize}
