# Supplementary material for: AExGym: Benchmarks and Environments for Adaptive Experimentation
Source: arXiv:2408.04531 source file (2024-08-08)
Supplement: Supplementary file 2 [file dataset-details.tex]

\section{Dataset Details}
\label{section:dataset_details}
As mentioned in section \ref{datasets}, we describe our data sources in more detail:
