# Supplementary material for: AExGym: Benchmarks and Environments for Adaptive Experimentation
Source: arXiv:2408.04531 source file (2024-08-08)
Supplement: Supplementary file 4 [file limitations.tex]

\section{Limitations}
\label{section:limitations}
While our simulation environment is able to provide functionalities not present in existing works, it also has limitations. First, we focus on providing an interface to convert publicly-available A/B test data and observational data into a bandit instance, rather than providing support for data collected from a bandit policy. As a result, we do not provide implementations of off-policy evaluation estimators for computing average policy rewards under a logging policy, as is done in ~\cite{saito2021open}. Nevertheless, these estimators can be seamlessly incorporated into our framework. Finally, while our framework allows for general agents, we limit our implementations to standard multi-armed and linear bandit and best-arm identification policies, due to their strong theoretical guarantees and relevance to settings faced by experimenters.
