# Supplementary material for: AExGym: Benchmarks and Environments for Adaptive Experimentation
Source: arXiv:2408.04531 source file (2024-08-08)
Supplement: Supplementary file 6 [file nonstationarity.tex]

\section{Nonstationarity}

Continued from Section \ref{experiments}, we further benchmark existing methods on the ASOS experiment and field experiment data.
