# Supplementary material for: AExGym: Benchmarks and Environments for Adaptive Experimentation
Source: arXiv:2408.04531 source file (2024-08-08)
Supplement: Supplementary file 8 [file policies.tex]

\section{Policies}
\label{section: policies}
