# Supplementary material for: AExGym: Benchmarks and Environments for Adaptive Experimentation
Source: arXiv:2408.04531 source file (2024-08-08)
Supplement: Supplementary file 9 [file site-selection.tex]

% \begin{table}[h!]
% \centering
% \begin{tabular}{lcccc}
% \toprule
%  & \textbf{profit} & \textbf{revenues} & \textbf{expenditures} & \textbf{consumption} \\
% \midrule
% Uniform & 0.537 & 0.761 & 0.483 & 0.751 \\
% TS & 0.638 & 0.777 & 0.487 & 0.777 \\
% TTTS & 0.572 & 0.842 & 0.582 & 0.804 \\
% UCB & 0.621 & 0.834 & 0.562 & 0.802 \\
% EI & 0.640 & 0.815 & 0.602 & 0.810 \\
% \bottomrule
% \end{tabular}
% \caption{Results from the Meager experiments when there are $64$ sequential rounds. }
% \label{tab:64-sites}
% \end{table}

\section{Site Selection}
\label{section:site-selection}

Recall the site selection task from from Section \ref{experiments}. In this section, we detail more experimental results from the Meager~\cite{Meager2019Understanding} and NHIS data~\cite{NHIS2010-2019}.
