# Supplementary material for: AExGym: Benchmarks and Environments for Adaptive Experimentation
Source: arXiv:2408.04531 source file (2024-08-08)
Supplement: Supplementary file 10 [file supplementary_material.tex]

\section*{Checklist}
